# Supplementary material for: Malleable Overview-Detail Interfaces
Source: arXiv:2503.07782 source file (2025-03-10)
Supplement: Supplementary file 2 [file 999_appendix.tex]

\clearpage
% \appendix
\section{Appendix}
\label{section:appendix}

\subsection{List of 33 categories from Semrush}
\label{appendix:semrush-categories}

\begin{itemize}
    \item Advertising and Marketing
    \item Airlines
    \item Apparel and Fashion
    \item Automotive
    \item Banking
    \item Beauty and Cosmetics
    \item Computer Software and Development
    \item Computer and Video Games
    \item Distance Learning
    \item Education
    \item Entertainment
    \item Finance
    \item Food and Beverages
    \item Gambling
    \item Healthcare
    \item Hospitality
    \item Human Resources
    \item Information Technology
    \item Insurance
    \item Investment
    \item Market Research
    \item Music
    \item Newspapers
    \item Online Services
    \item Real Estate
    \item Restaurants
    \item Retail
    \item Science
    \item Sports
    \item Telecom
    \item Transportation and Logistics
    \item Travel and Tourism
    \item Wellness
\end{itemize}
